# Supplementary material for: Tracking the Lithiation State of Li$_x$Si from Machine-Learned XPS Binding Energies
Source: arXiv:2602.23028 source file (2026-02-26)
Supplement: Supplementary file 1 [file supp-info.pdf]

# SUPPORTING INFORMATION

# Tracking the Lithiation State of $Li_xSi$ from Machine-Learned XPS Binding Energies

Michael Alejandro Hernandez Bertran,[†,‡] Davide Tisi,[¶] Federico Grasselli,[†,‡] Michele Ceriotti,[¶] Elisa Molinari,[†,‡] and Deborah Prezzi[*,‡]

†*Dipartimento di Scienze Fisiche, Informatiche, Matematiche (FIM), Università di Modena e Reggio Emilia, 41125 Modena, Italy*

‡*Nanoscience Institute, National Research Council (CNR-NANO), 41125 Modena, Italy*

¶*Laboratory of Computational Science and Modeling, Institut des Matériaux, École Polytechnique Fédérale de Lausanne, 1015 Lausanne, Switzerland*

E-mail: deborah.prezzi@cnr.it

## Model hyperparameters and learning curves

Figure S1 shows the overall accuracy of the ML models for the predicted Li 1$s$ (left) and Si 2$p$ (right) BEs, relative to ab initio DFT for the validation set. This is represented by the MAE in eV, as a function of both the characteristic distances $r_0$ used in the radial scaling of the SOAP descriptors and the number of local atomic environments in the training set. The effect of the different values of $r_0$ on the MAE is visible when considering $r_0$=5.5 Å and $r_0$=2.5 Å, which produce the larger and smaller MAE values, respectively. Regardless of the value of $r_0$, the prediction error continues to decrease with the inclusion of additional environments in the training set, without reaching a saturation regime. The optimal SOAP

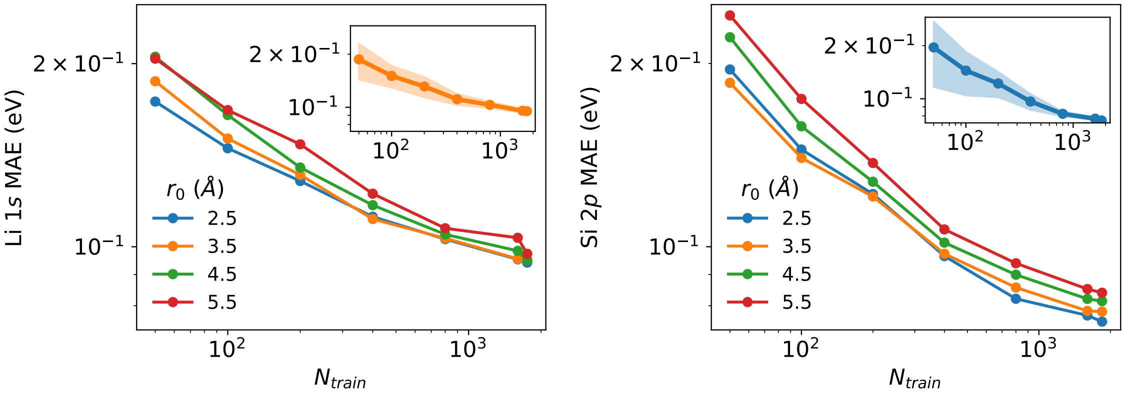


Figure S1: BE prediction error corresponding to the Li 1s (left) and Si 2p (right) models. The average MAE between the BEs predicted by the ML model and those obtained from DFT is shown on a log–log scale for different characteristic distances used in the radial scaling of the SOAP descriptor, as a function of the number of environments used for training $N_{train}$. For the selected characteristic distances an inset was added containing the average BE error (dot and line) with its uncertainty (shaded region) quantified as two times the standard deviation within the cross-validation folds.

and KRR Model parameters with the respective MAE and RMSE errors are reported in Table S1.

Table S1: **Optimal SOAP and Model parameters reported with their respective MAE and RMSE errors.**

| | **SOAP** | | **KRR** | | **Errors (eV)** | |
|---|---|---|---|---|---|---|
| **Core-level** | $r_0$ (Å) | $\sigma_a$ (Å) | $\lambda$ | $\gamma$ | MAE | RMSE |
| Li $1s$ | 3.5 | 0.3 | $2.98{\cdot}10^{-4}$ | 0.264 | 0.095 | 0.120 |
| Si $2p$ | 2.5 | 0.3 | $6.95{\cdot}10^{-5}$ | 0.379 | 0.075 | 0.096 |

# Evaluation of the Li $1s$ and Si $2p$ models on the Li$_x$Si dataset

In an amorphous solid, any observable $A$ could be evaluated as a canonical ensemble average over a large number of thermodynamically accessible static configurations $x_i$. If $A$ is defined as the binding energy value at which the XPS spectrum reaches its maximum intensity for

a given static configuration $x_i$, hereafter denoted $\text{BE}_{max}^{x_i}$, then its expected value over an amorphous $Li_xSi$ phase can be written as

$$\text{BE}_{max}^{x} = \langle \text{BE}_{max}^{x_i} \rangle_i = \sum_{i=1}^{N} \frac{e^{-\beta\varepsilon(x_i)}}{Z_x} \text{BE}_{max}^{x_i}, \quad (1)$$

where $N$ is the number of static configurations, or, in this case, structures, with the same Li concentration $x$, $\varepsilon(x_i)$ is the total energy per atom for the structure $x_i$ and $Z_x = \sum_{i=1}^{N} e^{-\beta\varepsilon(x_i)}$ is the partition function for the stoichiometry $x$.

Figure S2 shows $\text{BE}_{max}^{x}$ for the Li $1s$ (top) and Si $2p^{3/2}$ (bottom) XPS spectrum as a function of the Li concentration. The blue squares represent the values calculated using the ML predictions over the full $Li_xSi$ dataset[1] split in crystalline (left) and amorphous (right) structures, while the orange stars correspond to the values obtained from DFT calculations on the training set. The standard deviation for a given stoichiometry present in the dataset is represented by the blue area. For the Li $1s$ spectrum, no clear trend of $\text{BE}_{max}^{x}$ with respect to Li concentration is detected, neither for crystalline nor amorphous structures. In contrast, for the Si $2p^{3/2}$ spectrum, a clear downward trend of $\text{BE}_{max}^{x}$ is observed in both structural types, with marked jumps in the crystalline dataset within the $1<x<2$ region. For the a-$Li_xSi$ dataset, the $\text{BE}_{max}^{x}$ predicted by the model shows a smooth variation (except around $x \approx 2$) with a small error in the $0<x<1.5$ region. This trend is less apparent when using only the ab initio results from the training set, suggesting that convergence has not yet been achieved with respect to the number of static configurations used.

# Energetics and parameters convergence in grand canonical Monte Carlo simulations

Convergence tests were carried out on the BE values computed along the GCMC trajectories by reducing the acceptance ratio (from 44 to 27%, see Figure S3, left panel), and increasing

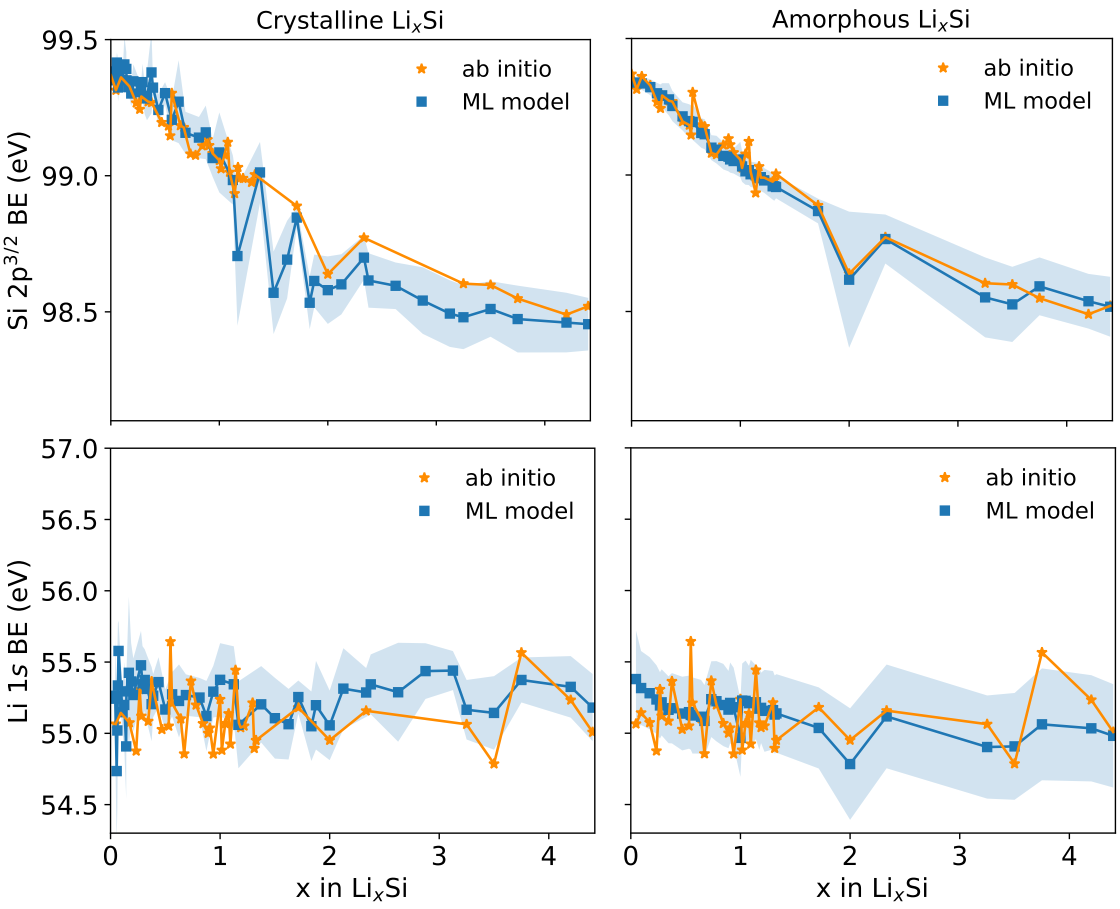


Figure S2: Stoichiometry maps showing the average peak position of Li 1$s$ (top) and Si $2p^{3/2}$ (bottom) for the c-$Li_x$Si (left) and a-$Li_x$Si (right) structures in the $Li_x$Si dataset. Blue squares represent ML model predictions, while orange stars denote ab initio calculations performed on the training set. The shaded blue region represents the standard deviation of the BEs for each stoichiometry.

the number of MD steps per MC move (from 50 to 100, see Figure S3, central panel). No significant changes were observed in the predicted BE values, confirming the robustness of the results with respect to the MC sampling. We observe instead a dependence on the system size (see Figure S3, right panel), and in particular, on the number of Si atoms required to obtain converged results in the region of low Li concentration. Importantly, convergence was only achieved for systems containing 8000 Si atoms (within an initial $Li_{3.75}Si$ cell of 76000 atoms).

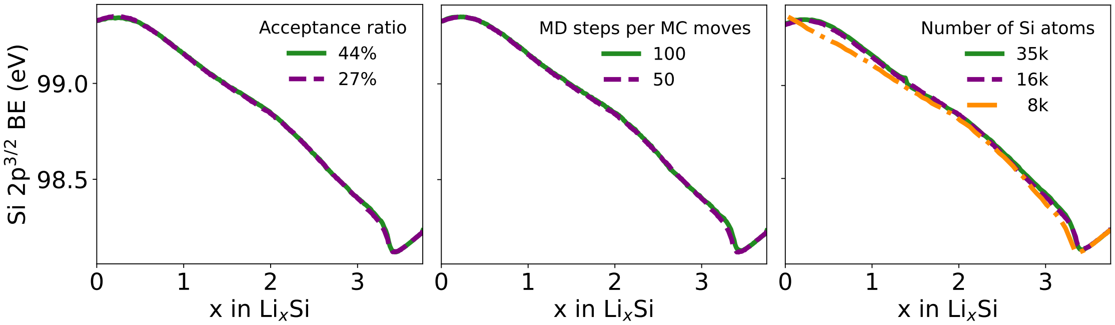


Figure S3: Convergence tests for the acceptance ratio (left), MD steps (center), and system size (right) performed for the GCMC simulation initiated from c-$Li_{3.75}Si$

# XPS Data Processing and Alignment Details

Experimental *ex situ* and *operando* XPS data were extracted from Ref. 2 and Ref. 3, respectively, using the PlotDigitizer software.[4] For a-Si thin films (30 nm in Ref. 2 and 95 nm in Ref. 3), Li diffusion is known to be sufficiently fast ($D_{Li} \approx 10^{-14} - 10^{-12} cm^2/s$)[5–9] to ensure nearly uniform Li distribution across the film thickness over the galvanostatic cycling times reported in these studies (≈1 h and ≈15 h for (de)lithiation, respectively). Under this hypothesis, we can consider the electrode potential as a reliable proxy for the approximated average Li content in the thin-film a-Si. Accordingly, the $BE_{max}$–$V$ data in Ref. 2 were mapped onto $BE_{max}$–$x$ using the corresponding lithiation state as a function of potential reported in Ref. 3. In addition, it is worth noting that Ref. 3 referenced all spectra to the

surface-hydrocarbon peak (C 1s region), while the spectra in Ref. 2 were provided without calibration. To enable a consistent comparison between the two experimental datasets and with our calculated BEs on a common reference scale, the $BE_{max}$ values from Ref. 3 were rigidly shifted to align their energy scale with that of Ref. 2 in the low-lithiation region. The different applied shifts ($\Delta E = 2.86$ eV for Li $1s$ and $\Delta E = 1.8$ eV for Si $2p$) reflect the fact that differential charging can lead to non-uniform offsets between core levels associated with distinct chemical environments.[10–14] Finally, since the Li $1s$ $BE_{\mathrm{max}}$ value corresponding to $Li_xSi$ was not explicitly reported in Ref. 2, the Li $1s$ spectrum was refitted in this work to isolate the contribution associated with the $Li_xSi$ phase, as illustrated in Figure S4.

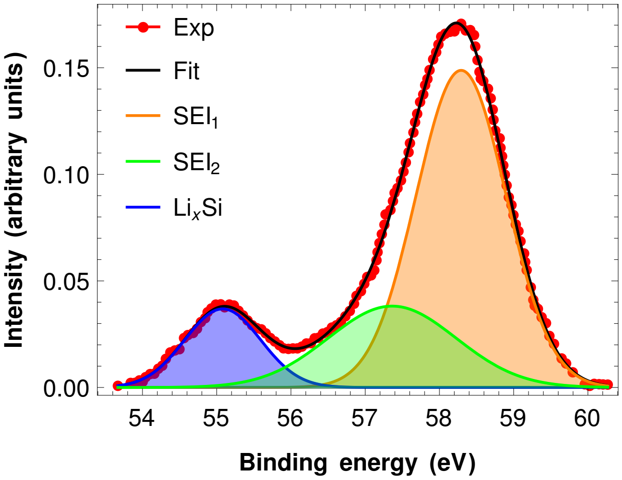


Figure S4: Example of the Li $1s$ curve-fitting result for Si electrode data at 0.07 V during delithiation, extracted from Ref. 2 (red points). The fitted components correspond to the various SEI species and the $Li_xSi$ contribution.

# Formation energy and convex hull from GCMC simulations

Figure S5 presents the formation energy per Si atom and the corresponding convex hull obtained from GCMC simulations starting at different Li concentrations. The convex hull represents the formation energy as a function of composition, where the envelope connects

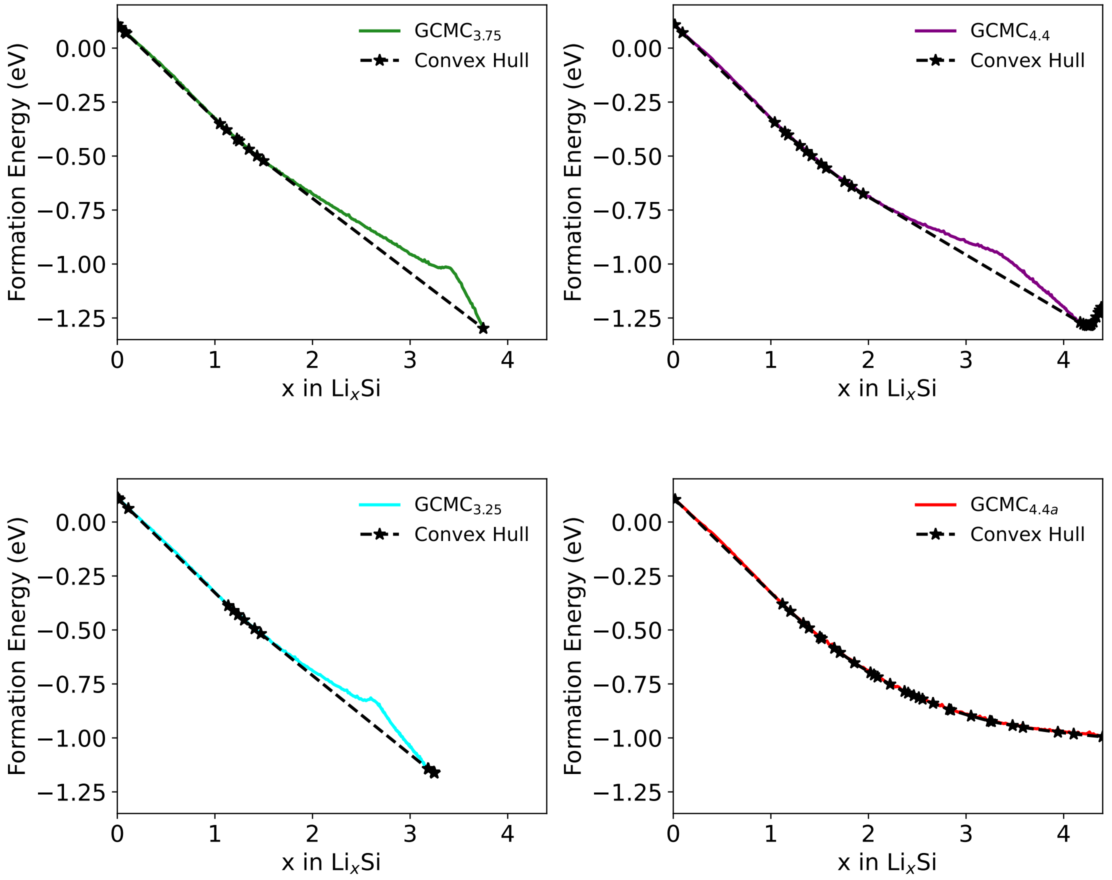


Figure S5: Formation energy per Si atom and convex hull from GCMC simulations starting from c-$Li_{3.75}Si$ (green), c-$Li_{4.4}Si$ (purple), a-$Li_{4.4}Si$ (red) and c-$Li_{3.25}Si$ (cyan).

the thermodynamically stable phases, bounding metastable and unstable phases above it. Furthermore, the slope of each line segment connecting adjacent points on the convex hull corresponds to the associated voltage value between the two phases.

Figure S6 shows the stoichiometry dependence of the Si $2p^{3/2}$ FWHM. In the low-Li concentration regime, the FWHM values obtained from the MQA (red solid line) and GCMC (green solid line) structures are in good agreement with each other and with *operando* experimental data[3] (black crosses). At $x \approx 3.4$, however, the experimental FWHM exhibits a characteristic peak associated with the amorphization of the c-$Li_{3.75}Si$ phase formed during lithiation. This feature is qualitatively reproduced only by the GCMC-generated structures, although shifted at higher concentrations, supporting the attribution to the crystal-to-amorphous transition.

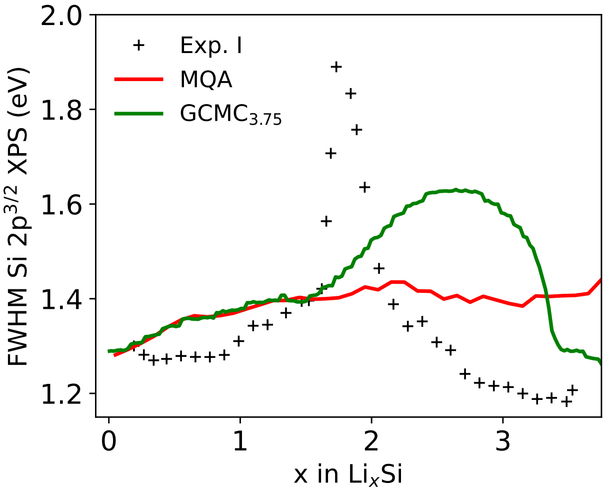


Figure S6: FWHM of Si $2p^{3/2}$ for $Li_xSi$ structures generated using MQA (red) and GCMC departing from c-$Li_{3.75}Si$ (green), compared to experimental data for Si electrodes from Ref. 3 (black crosses).

# References


(1) Fu, F.; Wang, X.; Zhang, L.; Yang, Y.; Chen, J. et al. Unraveling the Atomic-scale Mechanism of Phase Transformations and Structural Evolutions during (de)Lithiation

in Si Anodes. *Advanced Functional Materials* **2023**, *33*, 2303936.

(2) Ferraresi, G.; Czornomaz, L.; Villevieille, C.; Novák, P.; El Kazzi, M. Elucidating the Surface Reactions of an Amorphous Si Thin Film as a Model Electrode for Li-Ion Batteries. *ACS Applied Materials & Interfaces* **2016**, *8*, 29791–29798.

(3) Endo, R.; Ohnishi, T.; Takada, K.; Masuda, T. Electrochemical Lithiation and Delithiation in Amorphous Si Thin Film Electrodes Studied by Operando X-ray Photoelectron Spectroscopy. *The Journal of Physical Chemistry Letters* **2022**, *13*, 7363–7370.

(4) PlotDigitizer: Version 3.1.6. 2025; https://plotdigitizer.com.

(5) Hatchard, T. D.; Dahn, J. R. In Situ XRD and Electrochemical Study of the Reaction of Lithium with Amorphous Silicon. *Journal of The Electrochemical Society* **2004**, *151*, A838.

(6) Kulova, T.; Skundin, A.; Pleskov, Y.; Terukov, E.; Kon'kov, O. Lithium insertion into amorphous silicon thin-film electrodes. *Journal of Electroanalytical Chemistry* **2007**, *600*, 217–225, Equilibrium and kinetics of electrode processes.

(7) Ding, N.; Xu, J.; Yao, Y.; Wegner, G.; Fang, X. et al. Determination of the diffusion coefficient of lithium ions in nano-Si. *Solid State Ionics* **2009**, *180*, 222–225.

(8) Xie, J.; Imanishi, N.; Zhang, T.; Hirano, A.; Takeda, Y. et al. Li-ion diffusion in amorphous Si films prepared by RF magnetron sputtering: A comparison of using liquid and polymer electrolytes. *Materials Chemistry and Physics* **2010**, *120*, 421–425.

(9) Wang, J. W.; He, Y.; Fan, F.; Liu, X. H.; Xia, S. et al. Two-Phase Electrochemical Lithiation in Amorphous Silicon. *Nano Letters* **2013**, *13*, 709–715, PMID: 23323743.

(10) Metson, J. Charge compensation and binding energy referencing in XPS analysis. *Surface and Interface Analysis: An International Journal devoted to the development and*

*application of techniques for the analysis of surfaces, interfaces and thin films* **1999**, *27*, 1069–1072.

(11) Oswald, S. Binding energy referencing for XPS in alkali metal-based battery materials research (I): Basic model investigations. *Applied Surface Science* **2015**, *351*, 492–503.

(12) Baer, D. R.; Engelhard, M. H.; Gaspar, D. J.; Lea, A. S.; Windisch Jr, C. Use and limitations of electron flood gun control of surface potential during XPS: two non-homogeneous sample types. *Surface and Interface Analysis: An International Journal devoted to the development and application of techniques for the analysis of surfaces, interfaces and thin films* **2002**, *33*, 781–790.

(13) Suzer, S. Differential Charging in X-ray Photoelectron Spectroscopy: A Nuisance or a Useful Tool? *Analytical Chemistry* **2003**, *75*, 7026–7029, PMID: 14670067.

(14) Dubey, M.; Raman, A.; Gawalt, E. S.; Bernasek, S. L. Differential charging in X-ray photoelectron spectroscopy for characterizing organic thin films. *Journal of Electron Spectroscopy and Related Phenomena* **2010**, *176*, 18–23, Charging Issues in Electron Spectroscopies.
